# Supplementary material for: Consensus formation and relative stimulus perception in quality-sensitive, interdependent agent systems
Source: arXiv:2403.14856 ancillary file (2024-12-18)
Supplement: Supplementary file 1 [file SM.pdf]

# Supplementary Material for: Consensus formation and relative stimulus perception in quality-sensitive, interdependent agent systems

David March Pons,[1,*] Ezequiel E. Ferrero,[2,3,4] and M. Carmen Miguel[2,3]

[1]*Departament de Física, Universitat Politècnica de Catalunya, Campus Nord B4, 08034 Barcelona, Spain*
[2]*Departament de Física de la Matèria Condensada, Universitat de Barcelona, Martí i Franquès 1, 08028 Barcelona, Spain.*
[3]*Institute of Complex Systems (UBICS), Universitat de Barcelona, Barcelona, Spain*
[4]*Instituto de Nanociencia y Nanotecnología, CNEA–CONICET, Centro Atómico Bariloche, R8402AGP S. C. de Bariloche, Río Negro, Argentina.*

[*] david.march@upc.edu

TABLE I. Linear fit parameters obtained from the Weber's Law analysis (see Fig. 11 in the main text.). Quality differences have been fitted to $q_2 - q_1 = w\bar{q}$, where $\bar{q} = (q_1 + q_2)/2$ is the base quality or stimulus strength. The slope, $w$, represents the Weber's Fraction.

| $\lambda$ | $\pi_1, \pi_2$ | w | $R^2$ |
|---|---|---|---|
| 0.1 | 0.1, 0.1 | 0.4620 | 0.9985 |
| 0.3 | 0.1, 0.1 | 0.2398 | 0.9955 |
| 0.6 | 0.1, 0.1 | 0.0902 | 0.9960 |
| 0.9 | 0.1, 0.1 | 0.0168 | 0.9974 |
| 0.1 | 0.15, 0.05 | 1.0479 | 0.9980 |
| 0.3 | 0.15, 0.05 | 0.5694 | 0.9943 |
| 0.6 | 0.15, 0.05 | 0.2210 | 0.9956 |
| 0.9 | 0.15, 0.05 | 0.0417 | 0.9974 |

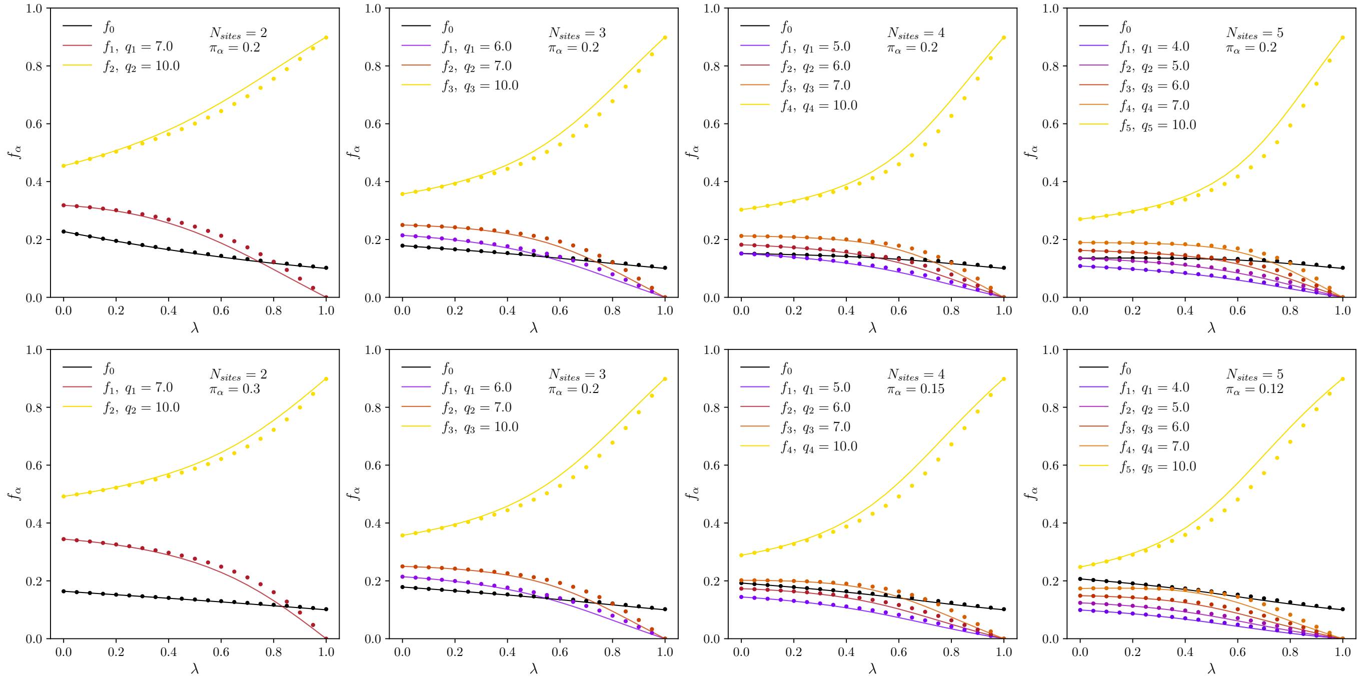


FIG. 1. Average dance frequencies $f_\alpha$ when increasing the number of sites, $k$. Lines indicate mean field results (obtained from numerical integration of Eqs.4) and dot markers indicate lattice simulations results. **Top row**: $\pi_\alpha = 0.2$ is maintained when increasing the number of sites. **Bottom row**: $\sum \pi_\alpha = 0.6$ is maintained when increasing the number of sites - consequently each individual value of $\pi_\alpha = 0.6/k$ is decreased. In any case the qualities are $q_k = 10$, $q_{k-1} = 7$, $q_{k-2} = 6$, ..., as indicated in the legend of each subplot.

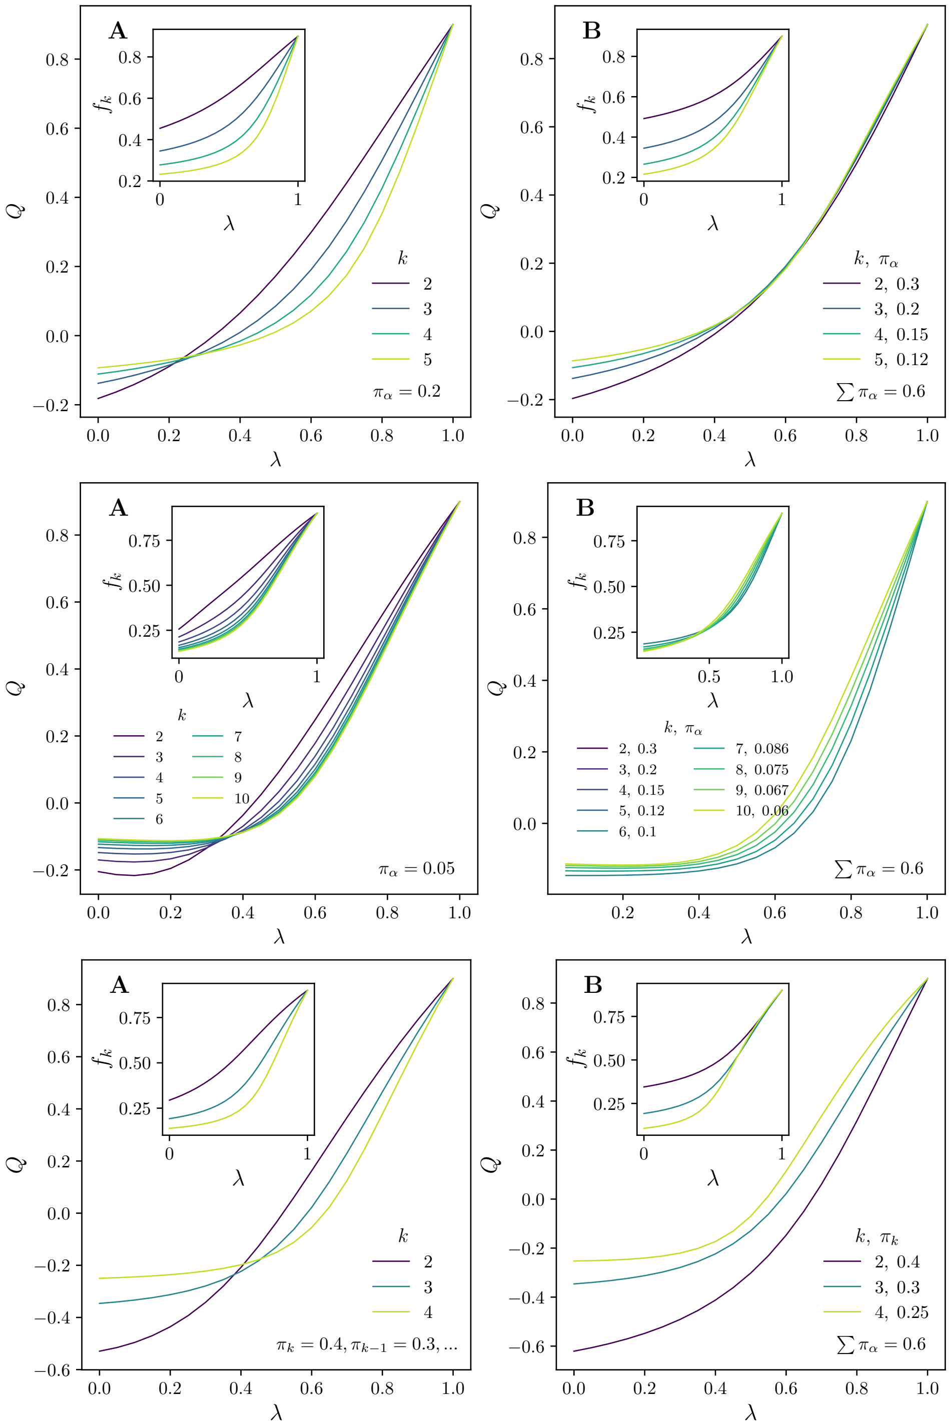


FIG. 2. Analytical results for the consensus and the population of the best quality site (inset) for scenarios beyond the binary decision problem. **Top row**: Considering up to $k = 5$ options in a symmetric discovery scenario with the same quality for the inferior options, $q_1 = ... = q_{k-1} = 7$, while $q_k = 10$. **Middle row**: Considering up to $k = 10$ sites in a symmetric discovery scenario with decreasing qualities ($q_k = 10$, $q_{k-1} = 9$, $q_{k-2} = 7...$). In both cases, left plots maintain $\pi_\alpha$ constant across sites ($\pi_\alpha = 0.2,\ 0.05$, respectively) while right plots maintain $\sum \pi_\alpha = 0.6$ constant, and thus $\pi_\alpha = 0.6/k$ values decrease when increasing the number of sites (see specific values in the legend). **Bottom row**: Considering up to $k = 4$ sites in an asymmetric discovery scenario with decreasing qualities ($q_k = 10$, $q_{k-1} = 7$, $q_{k-2} = 6...$). In the left plot, $\pi_k = 0.4$ and for each added site the discovery probabilities decrease by 0.1. In the right plot $\sum \pi_\alpha = 0.6$ is held constant, and thus the overall value of the $\pi_\alpha$ decreases; the legend states the discovery probability of the best quality option, $\pi_k$. Specifically, $\pi_\alpha$ values are $k = 2$: $((0.2, 0.4)$, $k = 3$: $(0.1, 0.2, 0.3)$ and $k = 4$: $(0.05, 0.12, 0.18, 0.25)$.
